# Supplementary material for: Let's Get Vysical: Perceptual Accuracy In Visual and Tactile Encodings
Source: arXiv:2308.04392 source file (2023-08-08)
Supplement: Supplementary file 1 [file Demographic_Questions.pdf]

# Demographic Questions

This document showcases questions asked before participants begin with the practice trials.

1. What is your age?
    a. 18-25
    b. 26-35
    c. 36-45
    d. 46-55
    e. 56-65
    f. 66-75
    g. 76-older
2. What is your gender?
    a. Male
    b. Female
    c. Other ______________
3. What is your ethnicity?
    a. American Indian or Alaska Native
    b. Asian
    c. Black or African American
    d. Hispanic
    e. Native Hawaiian or Other Pacific Islander
    f. White
    g. Two or More Races
    h. Other _______________
4. What is the highest level of education you completed?
    a. High school degree
    b. Associates degree
    c. College degree
    d. Masters' degree
    e. Doctorate
    f. Other
5. What is your occupation?
6. How familiar are you with data visualization concepts?
    a. Don't know what that is
    b. Somewhat familiar
    c. Moderately familiar
    d. Very familiar
    e. Extremely familiar
7. How much experience do you have in interpreting data visualizations?
    a. No experience
    b. Limited experience (less than a year)

    c. Some experience (1-2 years)
    d. Considerable experience (3-5 years)
    e. Extensive experience (more than 5 years)

8. On a scale of 1 to 5, with 1 being "not at all confident" and 5 being "extremely confident," how confident are you in your ability to read braille?
    a. Not at all confident
    b. Slightly confident
    c. Moderately confident
    d. Very confident
    e. Extremely confident
